# Supplementary material for: GreenMO: Virtualized User-proportionate MIMO
Source: arXiv:2211.16373 source file (2022-11-29)
Supplement: Supplementary file 1 [file appendix.tex]

\section{Appendix}~\label{app:appendix}

\subsection{Generalized $N$ antenna RF virtual chains}~\label{app:n-antenna}
Let us consider that the ADC is sampling at $NB$, and thus we will have $N$ $B$ bandwidth zones obtained from the ADC sampled stream $R$, denoted by $R^B_1, R^B_2, \ldots R^B_N = \mathbf{R^B}$, with $\mathbf{R^B}$ being a $N\times N_s$ matrix which stores the $N_s$ samples correpsonding to each of the $N$-th $B$ bandwidth zone, and we can obtain our virtualized RF chains $S_1,S_2,\ldots S_N = \mathbf{S}$, $S$ being $N \times N_s$ as well, via phase inversion of the $N\times N$ phase matrix $\mathbf{P}$ corresponding to the $j$-th harmonic phase of $c_i$:

\begin{equation}
    \mathbf{S} = (\mathbf{e}^{(-\mathbf{P})})* \mathbf{R^B}
\end{equation}

where $\mathbf{e}^{(\cdot)}$ applies the exponential function to each element of the matrix. The matrix $\mathbf{P}$ in detail looks like this:

\begin{equation*}
  \mathbf{P}=
  \begin{blockarray}{*{5}{c} l}
    \begin{block}{*{5}{>{$\footnotesize}c<{$}} l}
      0 & B & 2B & $\ldots$ & (N-1)B & \\
    \end{block}
    \begin{block}{[*{5}{c}]>{$\footnotesize}l<{$}}
      0 & 0 & 0 & $\ldots$ & 0 \bigstrut[t]& $c_1$ \\
      0 & \frac{2\pi}{N} & \frac{4\pi}{N} & $\ldots$ & \frac{2(N-1)\pi}{N} & $c_2$ \\
      $\ldots$ & $\ldots$ & $\ldots$ & $\ldots$ & $\ldots$ & $\ldots$ \\
      0 & \frac{2\pi(i-1)}{N} & \frac{4\pi(i-1)}{N} & $\ldots$ & \frac{2(N-1)(i-1)\pi}{N} & $c_i$ \\
      $\ldots$ & $\ldots$ & $\ldots$ & $\ldots$ & $\ldots$ & $\ldots$ \\
      0 & \frac{2\pi(N-1)}{N} & \frac{4\pi(N-1)}{N} & $\ldots$ & \frac{2(N-1)(N-1)\pi}{N} & $c_n$ \\
    \end{block}
  \end{blockarray}
\end{equation*}

\subsection{Algorithm to choose maximal set of antennas in-phase}~\label{app:babf}

This BABF algorithm chosen $\mathbf{B}$ creates a projected channel $\mathbf{HB}$ such that the remaining interference terms in $\mathbf{HB}$ can be handled easily by digital combining by be inverting this effective channel matrix via ZF approach as, $\mathbf{U} = \mathbf{(HB)}^{-1}\mathbf{S}$.

\begin{algorithm}
  \caption{BABF, Input: $\textbf{H}$, Output: $\mathbf{B}$}
  \begin{algorithmic}[1]
  \label{algo:switch_selection}
  \STATE $\phi$=$\pi/3$;\
  \FOR{ $1 \le i \le K$}{
      \FOR{ $1 \le m \le M$}{
      \STATE $\Tilde{\textbf{b}}_{i,m}=[0, 0 , \ldots , 0]_{1\times M}$;\
      \STATE $\textbf{g}_{i,m}=\textbf{H}_{i}h^*_{i,m}$;\
      \STATE $\boldsymbol{\theta}_{i,m}$=$\angle{\textbf{g}_{i,m}}$;\
      \STATE $\Tilde{\textbf{b}}_{i,m}(m)$=$|\boldsymbol{\theta}_{i,m}|<\frac{\pi}{4}$;\
      \STATE $score_{i,m}=$ Number of elements equal to $1$ in $\Tilde{\textbf{b}}_{i,m}$;
      }
      \ENDFOR
  }
  \ENDFOR
  \STATE $\mathbb{B} :=$ Set of all possible permutations of $score_{i,m}, 1 \le i \le K, 1 \le m \le M$\;
  \STATE $l=1$;\
  \STATE Select $score^*\in \mathbb{B}$ that provides the $l^{\text{th}}$ highest score;\
  \STATE $\mathbf{B}=\mathbf{B}^*$ (corresponding to $score^*$);\
  \IF{$\mathbf{H}\mathbf{B}$ is full rank}
  \STATE $\mathbf{B}$ is the optimal switch configuration;\
  \ELSE
  \STATE $l=l+1$;\
  \STATE Go to line 13;\
  \ENDIF
\end{algorithmic}
\label{Alg1}
\end{algorithm}
